# Supplementary material for: Don't Jump Through Hoops and Remove Those Loops: SVRG and Katyusha are Better Without the Outer Loop
Source: arXiv:1901.08689 source file (2019-06-05)
Supplement: Supplementary file 1 [file Loopless_NeurIPS2019_submission-11-14.pdf]

# Supplementary Material:

## SVRG and Katyusha are Better Without the Outer Loop

### A Auxiliary Lemmas

**Lemma A.1.** For random vector  $x \in \mathbb{R}^d$  and any  $y \in \mathbb{R}^d$ , the variance of  $y$  can be decomposed as

$$\mathbb{E} \left[ \|x - \mathbb{E}[x]\|^2 \right] = \mathbb{E} \left[ \|x - y\|^2 \right] - \mathbb{E} \left[ \|\mathbb{E}[x] - y\|^2 \right]. \quad (19)$$

The next lemma is a consequence of Jensen's inequality applied to  $x \mapsto \|x\|^2$ .

**Lemma A.2.** For any vectors  $a_1, a_2, \dots, a_k \in \mathbb{R}^d$ , the following inequality holds:

$$\left\| \sum_{i=1}^k a_i \right\|^2 \leq k \sum_{i=1}^k \|a_i\|^2. \quad (20)$$

### B Proofs for Algorithm 1 (L-SVRG)

In all proofs below, we will for simplicity write  $f^* \stackrel{\text{def}}{=} f(x^*)$ .

#### B.1 Proof of Lemma 3.1

Definition of  $x^{k+1}$  and unbiasedness of  $g^k$  guarantee that

$$\begin{aligned} \mathbb{E} \left[ \|x^{k+1} - x^*\|^2 \right] &= \mathbb{E} \left[ \|x^k - x^* - \eta g^k\|^2 \right] \\ &\stackrel{\text{Alg. 1}}{=} \|x^k - x^*\|^2 + \mathbb{E} \left[ 2\eta \langle g^k, x^* - x^k \rangle \right] + \eta^2 \mathbb{E} \left[ \|g^k\|^2 \right] \\ &\stackrel{(2)}{=} \|x^k - x^*\|^2 + 2\eta \langle \nabla f(x^k), x^* - x^k \rangle + \eta^2 \mathbb{E} \left[ \|g^k\|^2 \right] \\ &\stackrel{(4)}{\leq} \|x^k - x^*\|^2 + 2\eta \left( f^* - f(x^k) - \frac{\mu}{2} \|x^k - x^*\| \right) + \eta^2 \mathbb{E} \left[ \|g^k\|^2 \right] \\ &= \|x^k - x^*\|^2 (1 - \eta\mu) + 2\eta (f^* - f(x^k)) + \eta^2 \mathbb{E} \left[ \|g^k\|^2 \right]. \end{aligned}$$

#### B.2 Proof of Lemma 3.2

Using definition of  $g^k$

$$\begin{aligned} \mathbb{E} \left[ \|g^k\|^2 \right] &\stackrel{\text{Alg. 1}}{=} \mathbb{E} \left[ \|\nabla f_i(x^k) - \nabla f_i(x^*) + \nabla f_i(x^*) - \nabla f_i(w^k) + \nabla f(w^k)\|^2 \right] \\ &\stackrel{(20)}{\leq} 2\mathbb{E} \left[ \|\nabla f_i(x^k) - \nabla f_i(x^*)\|^2 \right] + 2\mathbb{E} \left[ \|\nabla f_i(x^*) - \nabla f_i(w^k) - \mathbb{E}[\nabla f_i(x^*) - \nabla f_i(w^k)]\|^2 \right] \\ &\stackrel{(3)+(19)}{\leq} 4L(f(x^k) - f^*) + 2\mathbb{E} \left[ \|\nabla f_i(w^k) - \nabla f_i(x^*)\|^2 \right] \\ &\stackrel{(8)}{=} 4L(f(x^k) - f^*) + \frac{p}{2\eta^2} \mathcal{D}^k. \end{aligned}$$

#### B.3 Proof of Lemma 3.3

$$\begin{aligned} \mathbb{E} \left[ \mathcal{D}^{k+1} \right] &\stackrel{\text{Alg. 1}}{=} (1-p)\mathcal{D}^k + p \frac{4\eta^2}{pn} \sum_{i=1}^n \|\nabla f(x^k) - \nabla f(x^*)\|^2 \\ &\stackrel{(3)}{\leq} (1-p)\mathcal{D}^k + 8L\eta^2(f(x^k) - f^*). \end{aligned}$$

## 308 **B.4 Proof of Lemma 3.4**

309 Combining Lemmas 3.1 and 3.3 we obtain

$$\begin{aligned}
\mathbb{E} \left[ \|x^{k+1} - x^*\|^2 + \mathcal{D}^{k+1} \right] &\stackrel{(9)+(11)}{\leq} (1 - \mu\eta) \|x^k - x^*\|^2 + 2\eta(f^* - f(x^k)) + \eta^2 \mathbb{E} \left[ \|g^k\|^2 \right] \\
&\quad + (1 - p)\mathcal{D}^k + 8L\eta^2(f(x^k) - f^*) \\
&\stackrel{(10)}{\leq} (1 - \mu\eta) \|x^k - x^*\|^2 + (1 - p)\mathcal{D}^k + (2\eta - 8L\eta^2)(f^* - f(x^k)) \\
&\quad + \eta^2 \left( 4L(f(x^k) - f^*) + \frac{p}{2\eta^2} \mathcal{D}^k \right) \\
&= (1 - \mu\eta) \|x^k - x^*\|^2 + \left( 1 - \frac{p}{2} \right) \mathcal{D}^k + (2\eta - 12L\eta^2)(f^* - f(x^k)).
\end{aligned}$$

310 Now we use the fact that  $\eta \leq \frac{1}{6L}$  and obtain the desired inequality:

$$\mathbb{E} \left[ \|x^{k+1} - x^*\|^2 + \mathcal{D}^{k+1} \right] \leq (1 - \mu\eta) \|x^k - x^*\|^2 + \left( 1 - \frac{p}{2} \right) \mathcal{D}^k.$$

## 311 **C Proofs for Algorithm 2 (L-Katyusha)**

### 312 **C.1 Proof of Lemma 4.1**

313 To upper bound the variance of  $g^k$  we first uses its definition

$$\begin{aligned}
\mathbb{E} \left[ \|g^k - \nabla f(x^k)\|^2 \right] &\stackrel{\text{Alg. 2}}{=} \mathbb{E} \left[ \left\| \nabla f_i(x^k) - \nabla f_i(w^k) - \mathbb{E} \left[ \nabla f_i(x^k) - \nabla f_i(w^k) \right] \right\|^2 \right] \\
&\stackrel{(19)}{\leq} \mathbb{E} \left[ \left\| \nabla f_i(x^k) - \nabla f_i(w^k) \right\|^2 \right] \\
&\stackrel{(3)}{\leq} 2L \left( f(w^k) - f(x^k) - \langle \nabla f(x^k), w^k - x^k \rangle \right).
\end{aligned}$$

### 314 **C.2 Proof of Lemma 4.2**

315 We start with the definition of  $z^{k+1}$

$$z^{k+1} \stackrel{\text{Alg. 2}}{=} \frac{1}{1 + \eta\sigma} \left( \eta\sigma x^k + z^k - \frac{\eta}{L} g^k \right),$$

316 which implies  $\frac{\eta}{L} g^k = \eta\sigma(x^k - z^{k+1}) + (z^k - z^{k+1})$ , which further implies that

$$\begin{aligned}
\langle g^k, z^{k+1} - x^* \rangle &= \mu \langle x^k - z^{k+1}, z^{k+1} - x^* \rangle + \frac{L}{\eta} \langle z^k - z^{k+1}, z^{k+1} - x^* \rangle \\
&= \frac{\mu}{2} \left( \|x^k - x^*\|^2 - \|x^k - z^{k+1}\|^2 - \|z^{k+1} - x^*\|^2 \right) \\
&\quad + \frac{L}{2\eta} \left( \|z^k - x^*\|^2 - \|z^k - z^{k+1}\|^2 - \|z^{k+1} - x^*\|^2 \right) \\
&\leq \frac{\mu}{2} \|x^k - x^*\|^2 + \frac{L}{2\eta} \left( \|z^k - x^*\|^2 - (1 + \eta\sigma) \|z^{k+1} - x^*\|^2 \right) - \frac{L}{2\eta} \|z^k - z^{k+1}\|^2.
\end{aligned}$$

317 **C.3 Proof of Lemma 4.3**

$$\begin{aligned}
& \frac{L}{2\eta} \|z^{k+1} - z^k\|^2 + \langle g^k, z^{k+1} - z^k \rangle \\
&= \frac{1}{\theta_1} \left( \frac{L}{2\eta\theta_1} \|\theta_1(z^{k+1} - z^k)\|^2 + \langle g^k, \theta_1(z^{k+1} - z^k) \rangle \right) \\
&\stackrel{\text{Alg. 2}}{=} \frac{1}{\theta_1} \left( \frac{L}{2\eta\theta_1} \|y^{k+1} - x^k\|^2 + \langle g^k, y^{k+1} - x^k \rangle \right) \\
&= \frac{1}{\theta_1} \left( \frac{L}{2\eta\theta_1} \|y^{k+1} - x^k\|^2 + \langle \nabla f(x^k), y^{k+1} - x^k \rangle + \langle g^k - \nabla f(x^k), y^{k+1} - x^k \rangle \right) \\
&= \frac{1}{\theta_1} \left( \frac{L}{2} \|y^{k+1} - x^k\|^2 + \langle \nabla f(x^k), y^{k+1} - x^k \rangle + \frac{L}{2} \left( \frac{1}{\eta\theta_1} - 1 \right) \|y^{k+1} - x^k\|^2 + \langle g^k - \nabla f(x^k), y^{k+1} - x^k \rangle \right) \\
&\stackrel{(3)}{\geq} \frac{1}{\theta_1} \left( f(y^{k+1}) - f(x^k) + \frac{L}{2} \left( \frac{1}{\eta\theta_1} - 1 \right) \|y^{k+1} - x^k\|^2 + \langle g^k - \nabla f(x^k), y^{k+1} - x^k \rangle \right) \\
&\geq \frac{1}{\theta_1} \left( f(y^{k+1}) - f(x^k) - \frac{\eta\theta_1}{2L(1-\eta\theta_1)} \|g^k - \nabla f(x^k)\|^2 \right) \\
&= \frac{1}{\theta_1} \left( f(y^{k+1}) - f(x^k) - \frac{\theta_2}{2L} \|g^k - \nabla f(x^k)\|^2 \right),
\end{aligned}$$

318 where the last inequality uses the Young's inequality in the form of  $\langle a, b \rangle \geq -\frac{\|a\|^2}{2\beta} - \frac{\beta\|b\|^2}{2}$  for  
319  $\beta = \frac{\eta\theta_1}{L(1-\eta\theta_1)}$ , which concludes the proof.

320 **C.4 Proof of Lemma 4.4**

321 From the definition of  $w^{k+1}$  in Algorithm 2 we have

$$\mathbb{E} [f(w^{k+1})] \stackrel{\text{Alg. 2}}{=} (1-p)f(w^k) + pf(y^k). \quad (21)$$

322 The rest of proof follows from the definition of  $\mathcal{W}^k$  (17).

323 **C.5 Proof of Lemma 4.5**

324 Combining all the previous lemmas together, we obtain

$$\begin{aligned}
f^* &\stackrel{(4)}{\geq} f(x^k) + \langle \nabla f(x^k), x^* - x^k \rangle + \frac{\mu}{2} \|x^k - x^*\|^2 \\
&= f(x^k) + \frac{\mu}{2} \|x^k - x^*\|^2 + \langle \nabla f(x^k), x^* - z^k + z^k - x^k \rangle \\
&\stackrel{\text{Alg. 2}}{=} f(x^k) + \frac{\mu}{2} \|x^k - x^*\|^2 + \langle \nabla f(x^k), x^* - z^k \rangle + \frac{\theta_2}{\theta_1} \langle \nabla f(x^k), x^k - w^k \rangle + \frac{(1 - \theta_1 - \theta_2)}{\theta_1} \langle \nabla f(x^k), x^k - y^k \rangle \\
&\stackrel{(2)}{\geq} f(x^k) + \frac{\theta_2}{\theta_1} \langle \nabla f(x^k), x^k - w^k \rangle + \frac{(1 - \theta_1 - \theta_2)}{\theta_1} (f(x^k) - f(y^k)) \\
&\quad + \mathbb{E} \left[ \frac{\mu}{2} \|x^k - x^*\|^2 + \langle g^k, x^* - z^{k+1} \rangle + \langle g^k, z^{k+1} - z^k \rangle \right] \\
&\stackrel{(15)}{\geq} f(x^k) + \frac{\theta_2}{\theta_1} \langle \nabla f(x^k), x^k - w^k \rangle + \frac{(1 - \theta_1 - \theta_2)}{\theta_1} (f(x^k) - f(y^k)) \\
&\quad + \mathbb{E} \left[ \mathcal{Z}^{k+1} - \frac{1}{1 + \eta\sigma} \mathcal{Z}^k \right] + \mathbb{E} \left[ \langle g^k, z^{k+1} - z^k \rangle + \frac{L}{2\eta} \|z^k - z^{k+1}\|^2 \right] \\
&\stackrel{(16)}{\geq} f(x^k) + \frac{\theta_2}{\theta_1} \langle \nabla f(x^k), x^k - w^k \rangle + \frac{(1 - \theta_1 - \theta_2)}{\theta_1} (f(x^k) - f(y^k)) \\
&\quad + \mathbb{E} \left[ \mathcal{Z}^{k+1} - \frac{1}{1 + \eta\sigma} \mathcal{Z}^k \right] + \mathbb{E} \left[ \frac{1}{\theta_1} (f(y^{k+1}) - f(x^k)) - \frac{\theta_2}{2L\theta_1} \|g^k - \nabla f(x^k)\|^2 \right] \\
&\stackrel{(14)}{\geq} f(x^k) + \frac{\theta_2}{\theta_1} \langle \nabla f(x^k), x^k - w^k \rangle + \frac{(1 - \theta_1 - \theta_2)}{\theta_1} (f(x^k) - f(y^k)) \\
&\quad + \mathbb{E} \left[ \mathcal{Z}^{k+1} - \frac{1}{1 + \eta\sigma} \mathcal{Z}^k \right] + \mathbb{E} \left[ \frac{1}{\theta_1} (f(y^{k+1}) - f(x^k)) - \frac{\theta_2}{\theta_1} (f(w^k) - f(x^k) - \langle \nabla f(x^k), w^k - x^k \rangle) \right] \\
&= f(x^k) + \frac{(1 - \theta_1 - \theta_2)}{\theta_1} (f(x^k) - f(y^k)) - \frac{1}{1 + \eta\sigma} \mathcal{Z}^k - \frac{\theta_2}{\theta_1} (f(w^k) - f(x^k)) \\
&\quad + \mathbb{E} \left[ \mathcal{Z}^{k+1} + \frac{1}{\theta_1} (f(y^{k+1}) - f(x^k)) \right],
\end{aligned}$$

325 where in the second inequality we use also convexity of  $f(x)$ .

$$\begin{aligned}
x^k &\stackrel{\text{Alg. 2}}{=} \theta_1 z^k + \theta_2 w^k + (1 - \theta_1 - \theta_2) y^k \\
z^k - x^k &= \frac{\theta_2}{\theta_1} (x^k - w^k) + \frac{1 - \theta_1 - \theta_2}{\theta_1} (x^k - y^k).
\end{aligned}$$

326 After rearranging we get

$$\frac{1}{1 + \eta\sigma} \mathcal{Z}^k + (1 - \theta_1 - \theta_2) \mathcal{Y}^k + \frac{\theta_2}{\theta_1} (f(w^k) - f^*) \geq \mathbb{E} [\mathcal{Z}^{k+1} + \mathcal{Y}^{k+1}].$$

327 Using definition of  $\mathcal{W}^k$  we get

$$\mathbb{E} [\mathcal{Z}^{k+1} + \mathcal{Y}^{k+1}] \leq \frac{1}{1 + \eta\sigma} \mathcal{Z}^k + (1 - \theta_1 - \theta_2) \mathcal{Y}^k + \frac{p}{(1 + \theta_1)} \mathcal{W}^k. \quad (22)$$

328 Finally, using Lemma 4.4 we get

$$\begin{aligned}
\mathbb{E} [\mathcal{Z}^{k+1} + \mathcal{Y}^{k+1} + \mathcal{W}^{k+1}] &\leq \frac{1}{1 + \eta\sigma} \mathcal{Z}^k + (1 - \theta_1 - \theta_2) \mathcal{Y}^k + \frac{p}{(1 + \theta_1)} \mathcal{W}^k + (1 - p) \mathcal{W}^k + \theta_2 (1 + \theta_1) \mathcal{Y}^k \\
&= \frac{1}{1 + \eta\sigma} \mathcal{Z}^k + (1 - \theta_1 (1 - \theta_2)) \mathcal{Y}^k + \left( 1 - \frac{p\theta_1}{1 + \theta_1} \right) \mathcal{W}^k,
\end{aligned}$$

329 which concludes the proof.
